# Supplementary material for: Error per single-qubit gate below $10^{-4}$ in a superconducting qubit
Source: arXiv:2302.08690 ancillary file (2023-02-17)
Supplement: Supplementary file 1 [file Suppl.pdf]

# Supplemental Material for: Error per single-qubit gate below $10^{-4}$ in a superconducting qubit

Zhiyuan Li,[1,*] Pei Liu,[2,*] Peng Zhao,[1] Zhenyu Mi,[1] Huikai Xu,[1] Xuehui Liang,[1] Tang Su,[1] Weijie Sun,[1] Guangming Xue,[1] Jing-Ning Zhang,[1,†] Weiyang Liu,[1,‡] Yirong Jin,[1] and Haifeng Yu[1]

[1] *Beijing Academy of Quantum Information Sciences, Beijing 100193, China*
[2] *State Key Laboratory of Low Dimensional Quantum Physics, Department of Physics, Tsinghua University, Beijing 100084, China*

(Dated: February 16, 2023)

## I. READOUT CALIBRATION AND QUBIT COHERENCE CHARACTERIZATION

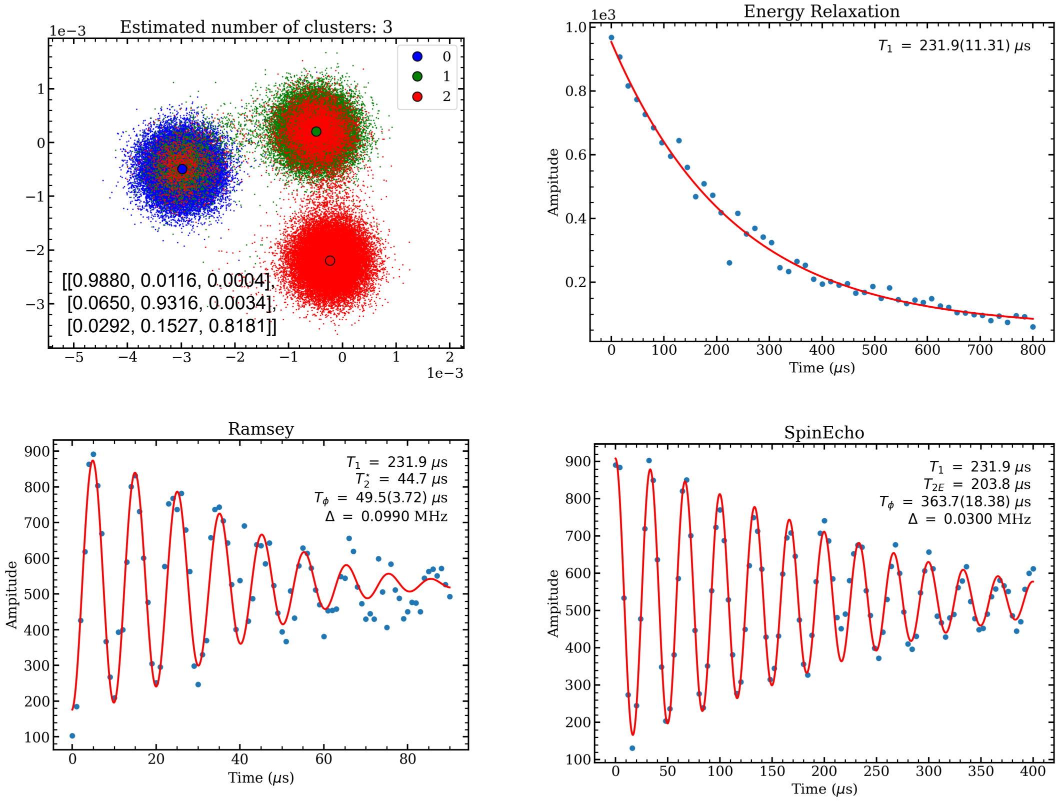


FIG. S1. (a) Single shot measurement events for the qubit in $|0\rangle$, $|1\rangle$ and $|2\rangle$ state of $Q_5$. (b)The relaxation of $Q_5$. (c) The Ramsey data of $Q_5$. (d) The spin echo data of $Q_5$.

In Figure S1 (a), we show In-phase and quadrature (IQ) components of the dispersed signal with the qubit prepared in $|0\rangle$, $|1\rangle$ and $|2\rangle$ state. The readout microwave signal is pre-amplified by a High-Electron-Mobility Transistor at the 4K stage. Further amplified by two microwave amplifiers at room temperature, then down-converted to IQ signals. The insert is the readout transition matrix, which is used to correct the qubit multi-state probability. Figure S1 (b)-(d) are the average relaxation time, Ramsey interferometry, and spin echo results, respectively.

---

* Z. Li and P. Liu contributed equally to this work.
† Corresponding author: zhangjn@baqis.ac.cn
‡ Corresponding author: liuwy@baqis.ac.cn

## II. MODEL VIOLATION WITH QUANTUM STATE TOMOGRAPHY

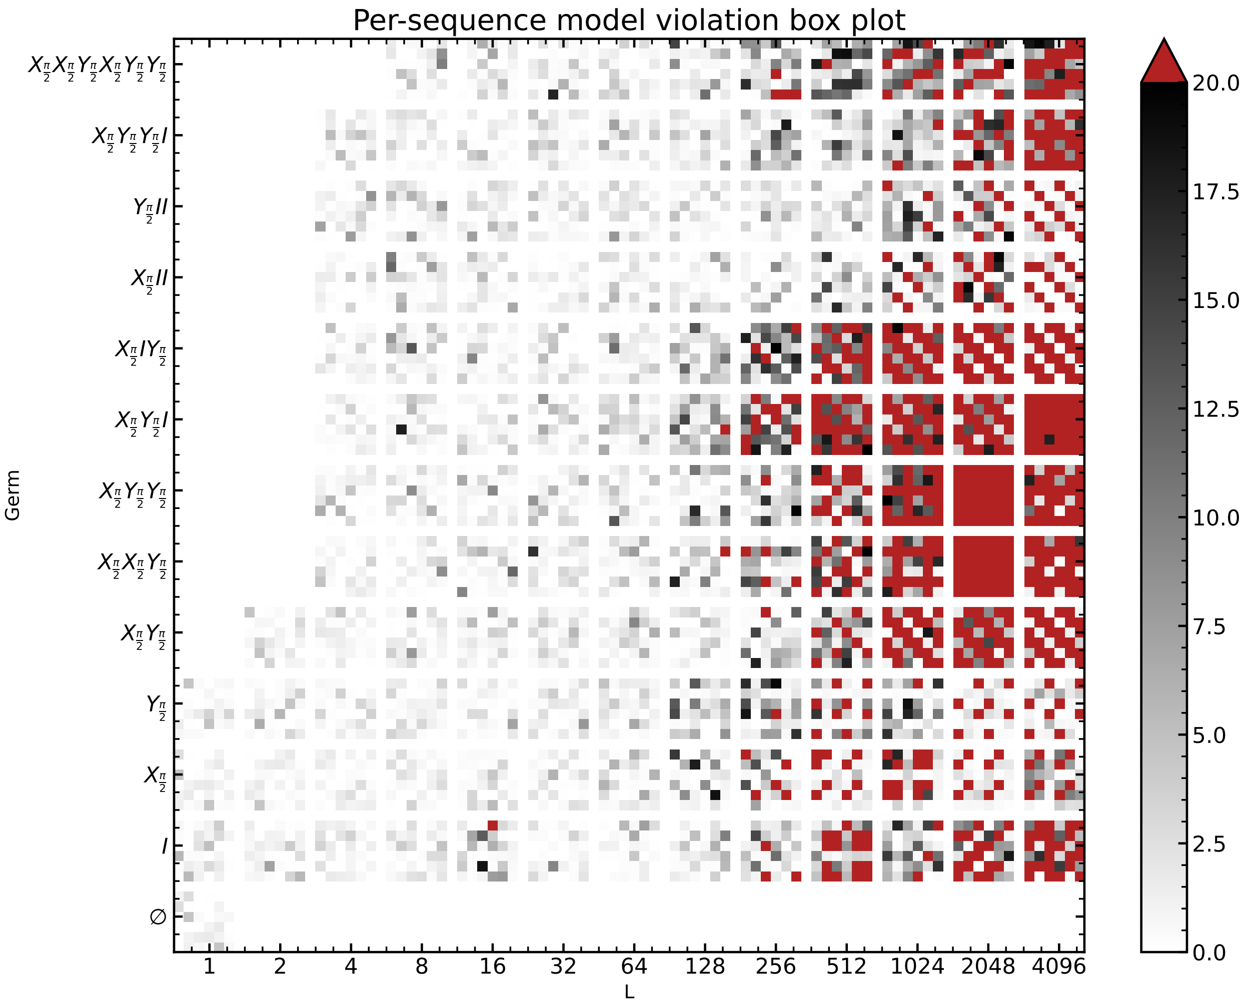


FIG. S2. Model violation for each circuit. When the circuit length increases, the experiment outcomes are inconsistent with the Markovian model at 95% confidence level. When the outcomes exceed this bound, the box will be red.

## III. THE INSTABILITY OF PARAMETERS

To examine the stability of the qubit frequency, we perform the long-term measurements of Ramsey. The frequency fluctuations $\Delta\omega_q$ and the power spectral density of frequency fluctuations are shown in Figure S3 (a) and (b) [1].

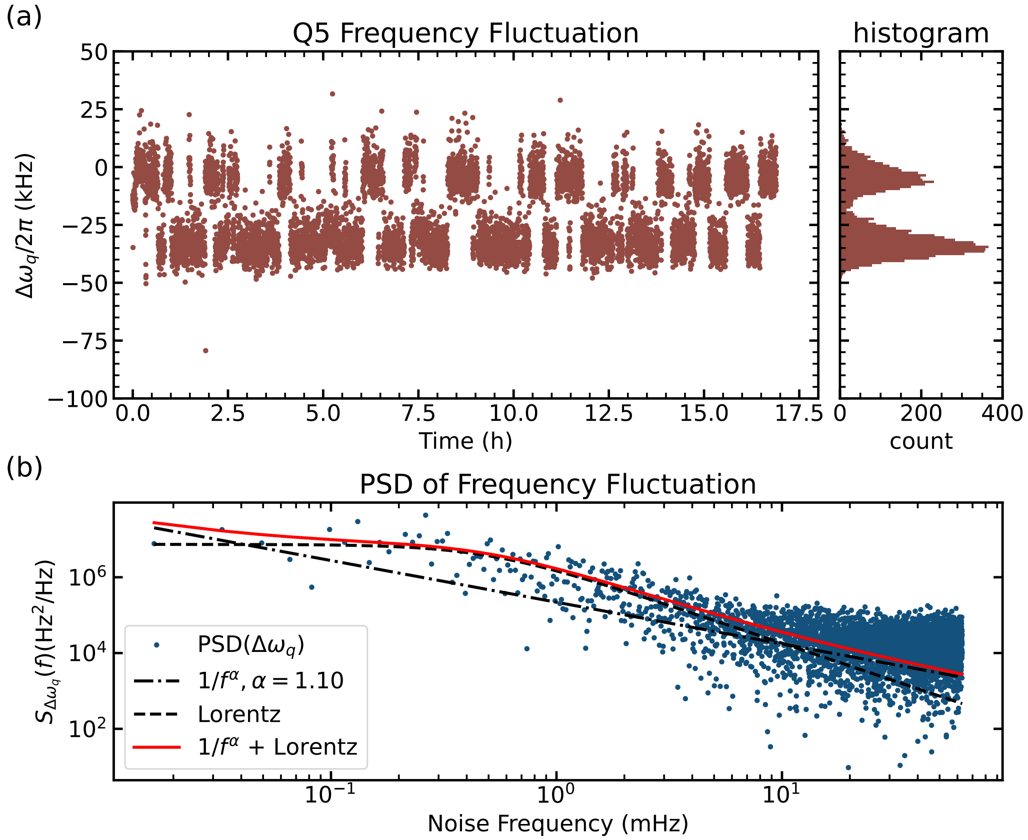


FIG. S3. (a) Data taken over 17 hours displays fluctuations of the qubit frequency, telegraph-like switching of the qubit frequency $\Delta\omega_q$. (b) The power spectral density of frequency fluctuations. The noise looks like telegraphic noise and $1/f^{\alpha}$ noise.

We perform the long-term measurements of Rabi. The fluctuations and the power spectral density of pulse amplitude are shown in Figure S4 (a) and (b).

[1] S. Schlör, J. Lisenfeld, C. Müller, A. Bilmes, A. Schneider, D. P. Pappas, A. V. Ustinov, and M. Weides, Physical Review Letters **123**, 190502 (2019).

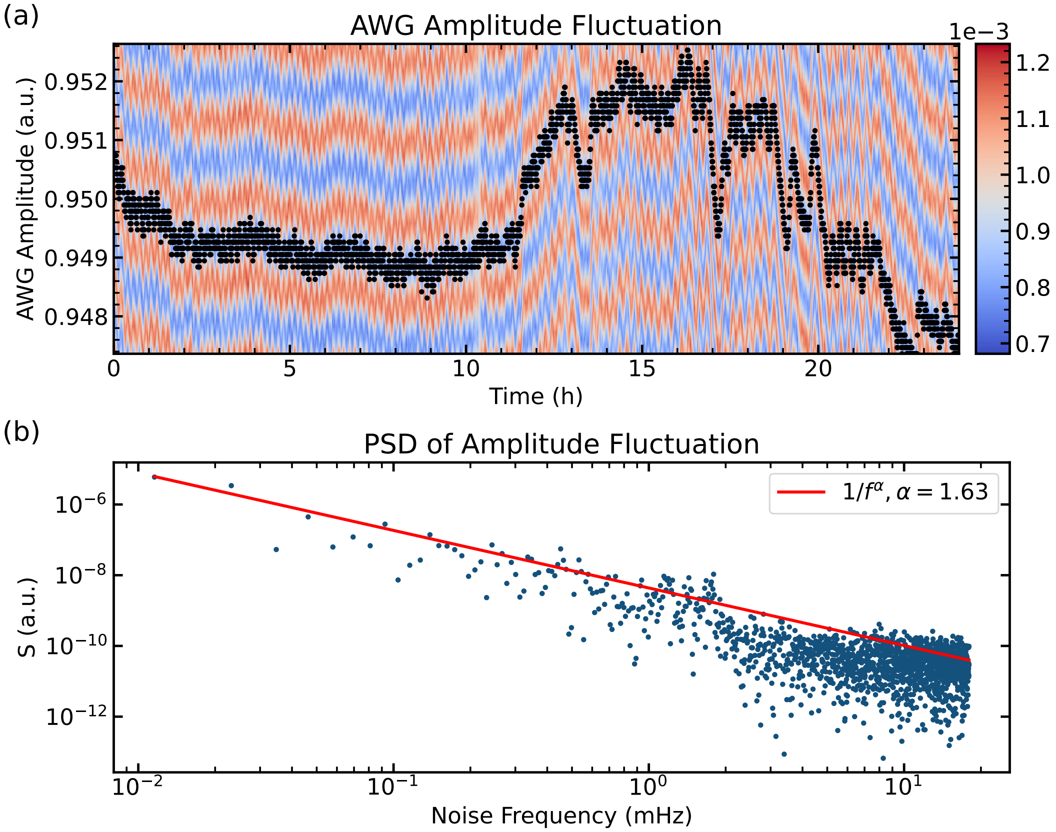


FIG. S4. (a) A quantum circuit composed of the total 1801 $X_\pi$ detect the fluctuations of the AWG amplitude. The dark line shows the instability over 24 hours. (b) The noise spectrum of AWG amplitude extracted from (a). The noise is close to 1/f noise.
